# Supplementary material for: When Dynamic Data Selection Meets Data Augmentation
Source: arXiv:2505.03809 source file (2025-05-02)
Supplement: Supplementary file 1 [file appendix.tex]

\appendix
\onecolumn
\section{More Implementation Details}

\subsection{Augmentation Space}
\begin{table}[h]
    \centering
    \caption{Augmentation operations and their magnitudes.}
    \label{tab:augmentation_ops}
    \begin{tabular}{l|c|c}
        \toprule
        \textbf{Operation} & \textbf{Value Range} & \textbf{Magnitude-based} \\
        \midrule
        Identity & - & \texttimes \\
        ShearX & $[0.0, 0.99]$ & \checkmark \\
        ShearY & $[0.0, 0.99]$ & \checkmark \\
        TranslateX & $[0.0, 32.0]$ & \checkmark \\
        TranslateY & $[0.0, 32.0]$ & \checkmark \\
        Rotate & $[0.0, 135.0]$ & \checkmark \\
        Brightness & $[0.0, 0.99]$ & \checkmark \\
        Color & $[0.0, 0.99]$ & \checkmark \\
        Contrast & $[0.0, 0.99]$ & \checkmark \\
        Sharpness & $[0.0, 0.99]$ & \checkmark \\
        Posterize & $[2, 8]$  & \checkmark \\
        Solarize & $[255.0, 0.0]$ & \checkmark \\
        AutoContrast & - & \texttimes \\
        Equalize & - & \texttimes \\
        \bottomrule
    \end{tabular}
\end{table}

\subsection{Fine-tuning the Adapters}
The adapter is one linear layer. During the fine-tuning process, the weights of entire CLIP models are frozen.
Due to the lightweight design of the adapters with small parameter sizes, fine-tuning can be completed efficiently.
Specifically, we use the learning rate of $1e-4$, an Adam optimizer, and the decay factor of 0.1.
On ImageNet-1k, the total epoch is 10, and the batch size is 512, while on other datasets, the total epoch is 20 with a batch size of 256.

% \section{The Specific Algorithm Workflow}
% The detailed algorithm is summarized in Algorithm~\ref{alg}.
% \begin{algorithm}[h]
% \begin{algorithmic}[1]
%     \caption{The general workflow.}\label{alg}
%     \REQUIRE dataset $D$, image and text feature embedding
%     \ENSURE selected $\hat{D}_{t+1}$ for epoch $t+1$
% \end{algorithmic}
% \end{algorithm}

\section{Illustrations of Corrupted Images}
In this section, we provide the illustrations of corrupted images in Figure~\ref{fig-examples}.
\begin{figure}[h]
    \centering
        \subfloat[Origin]{\label{fig5-1}
 		\centering
 		\includegraphics[width=.12\textwidth]{./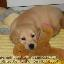}}
         \subfloat[fog]{\label{fig5-2}
 		\centering
 		\includegraphics[width=.12\textwidth]{./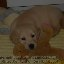}}
        \subfloat[Gaussian]{\label{fig5-3}
 		\centering
 		\includegraphics[width=.12\textwidth]{./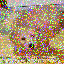}}
        \subfloat[motion blur]{\label{fig5-3}
 		\centering
 		\includegraphics[width=.12\textwidth]{./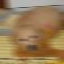}}
        \subfloat[Occlusion]{\label{fig5-3}
 		\centering
 		\includegraphics[width=.12\textwidth]{./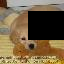}}
        \subfloat[Resolution]{\label{fig5-3}
 		\centering
 		\includegraphics[width=.12\textwidth]{./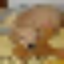}}
\caption{Illustration of the image corruption types, including fog, Gaussian noise, motion blur, random occlusion, and resolution.}
\label{fig-examples}
\end{figure}

\section{Discussion and Future Work}
In this paper, we propose a novel online data training framework that unifies dynamic data selection and data augmentation to achieve enhanced model training acceleration.
In this section, we discuss some potential limitations and future work for our method.
1). Our proposed method is based on the pretrained CLIP model to estimate the sample semantic consistency. 
While this exhibits superior effectiveness in general datasets, further applying our method to special tasks, such as medical imaging, where pretrained multimodal models are unavailable or mismatched, is worth exploring in future work.
2). We employ our framework on image classification tasks and demonstrate its superior effectiveness. Future work should extend the applications to more real-world tasks, such as object detection and segmentation.
